# Supplementary material for: Simple yet Effective Gradient-Free Graph Convolutional Networks
Source: arXiv:2302.00371 source file (2023-02-01)
Supplement: Supplementary file 1 [file supplement.pdf]

# Simple yet Effective Gradient-Free Graph Convolutional Networks Supplement

## A Dataset Statistics

An overview summary of the datasets used in our experiments is given in Tab. 1.

Table 1: Details of the datasets.

| Dataset | #Nodes | #Edges | #Features | #Classes |
|---|---|---|---|---|
| Cora | $2,708$ | $5,429$ | $1,433$ | 7 |
| Cora-ML | $2,995$ | $8,416$ | $2,879$ | 7 |
| Citeseer | $3,327$ | $4,732$ | $3,703$ | 6 |
| PubMed | $19,717$ | $44,338$ | 500 | 3 |

## B More Model Setting

For GCNII, we set the strength of the initial residual connection $\alpha = 0.1$ and the strength of the identity mapping $\theta = 0.5$. We set the graph convolutional layer as 16 units. For our methods, we tune the hyperparameter $\lambda$ in Eqn. (17) based on the evaluation of the validation set (Referring to Sec. D in the supplement). We also tune the weight decay for all the baselines with grid search ranged in $[10^{-8}, 10^{-3}]$.

## C Vanishing Gradient of Linearized GCN

### C.1 Analysis for SGC

For SGC, we have

$$\lim_{K\to\infty} \left(\mathcal{F}_G - \tfrac{1}{N}\mathbf{1}_N\mathbf{1}_N^\top\mathcal{F}_G\right) = \mathbf{0}. \tag{1}$$

which is small, if $\tau$ is small.

*Proof.* If the graph is connected and not bipartite, the greatest eigenvalue of row-normalized adjacency matrix $\mathbf{A}_{\text{rw}}$ is 1, and the corresponding eigenvector is $\mathbf{1}_N$. All eigenvalues of $\mathbf{A}_{\text{rw}}$ other than 1 falls into the range $(-1, 1)$. For SGC, when $K$ approximates $+\infty$, only component of eigenvector $\mathbf{1}_N$ in $\mathbf{X}$ is reserved. As a result,

$$\lim_{K\to\infty} \mathcal{F}_G = \lim_{K\to\infty} \mathbf{A}_{rw}^K\mathbf{X} = \theta\mathbf{1}_N\mathbf{1}_C^\top. \tag{2}$$

Given Eqn. (2), it is easy to verify that Eqn. (2) holds. □

### C.2 Analysis for SSGC

For SSGC, we have

$$\lim_{K\to\infty} \left(\mathcal{F}_G - \tfrac{1}{N}\mathbf{1}_N\mathbf{1}_N^\top\mathcal{F}_G\right) = \tau\left(\mathbf{X} - \tfrac{1}{N}\mathbf{1}_N\mathbf{1}_N^\top\mathbf{X}\right), \tag{3}$$

*Proof.* For SSGC, we have

$$\mathcal{F}_G = \tau\mathbf{X} + (1-\tau)\frac{1}{K}\sum_{k=1}^{K}\mathbf{A}_{rm}^k\mathbf{X}. \tag{4}$$

By Eqn. (2),

$$\lim_{K\to\infty} \mathcal{F}_G = \tau\mathbf{X} + (1-\tau)\theta\mathbf{1}_N\mathbf{1}_C^\top. \tag{5}$$

Thus, Eqn (3) holds. The right side of (3) is just the zero-centered $\tau\mathbf{X}$. □

### C.3 Analysis for DGC

For DGC, we have

$$\lim_{K\to\infty} \left(\mathcal{F}_G - \tfrac{1}{N}\mathbf{1}_N\mathbf{1}_N^\top\mathcal{F}_G\right) \tag{6}$$

$$= (I - \tfrac{1}{N}\mathbf{1}_N\mathbf{1}_N^\top)\exp(T(\mathbf{A}_{rw} - I))\mathbf{X}, \tag{7}$$

which is small, when $T$ is large.

*Proof.* For DGC, $\mathcal{F}_G = \mathbf{A}_{dgc}^K\mathbf{X}$, where

$$\mathbf{A}_{dgc} = \left(1 - \tfrac{T}{K}\right)I + \tfrac{T}{K}\hat{\mathbf{A}}_{rw}. \tag{8}$$

When $K$ approximate $+\infty$,

$$\lim_{K\to\infty} \mathbf{A}_{dgc}^K = \exp(T(\mathbf{A} - I)), \tag{9}$$

where $\exp(\cdot)$ is matrix exponential. And, zero-centered $\mathcal{F}_G$ approximates

$$\lim_{K\to\infty} \mathcal{F}_G = \exp(T(\mathbf{A} - I))\mathbf{X}. \tag{10}$$

Thus, Eqn. (6) holds. □

## D Sensitivity Analysis

To validate the hyperparameter $\lambda$'s impact on our gradient-free framework, we propose the sensitivity analysis and target on the SGC backbones as an exemplar on the Cora dataset. We fix $K = 2, 8, 32, 128$ to represent the sensitivity analysis under different levels of depth. The experiment results

are shown in Fig. 1. It demonstrates that the node classification performance of gfSGC is sensitive to the choice of $\lambda$. It makes sense since almost all the graphs' features are highly dimensional, it is vital to appropriately prune redundant information to boost the gfSGC's performance. Another important finding is that gfSGC behaves differently with varying depths. The trend is that as $K$ increases, the optimal $\lambda$ tends to be a smaller value. It is maybe the increasing receptive field caused by the increasing $K$ that will provide more important semantic information to each node. As a result, we should add less penalty on the sparsity of weights.

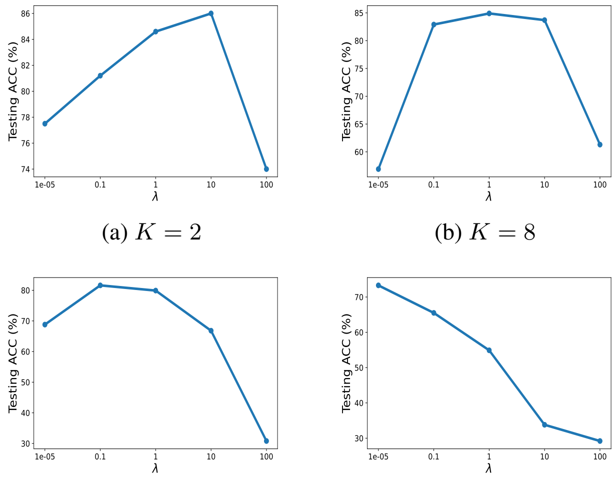


(a) $K = 2$ (b) $K = 8$

(c) $K = 32$ (d) $K = 128$

Figure 1: Node classification performance of gfSGC on Cora with varying $\lambda$ and $K$.

# E Vanishing Gradient of DGC

Theorem 1 mentioned that when $T$ is large, DGC will encounter the vanishing gradient. We present the gradient density plot of DGC with varying $T$ for $K = 64$ and $K = 128$ as exemplar in Fig. 2.

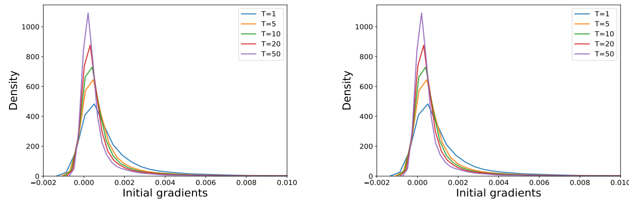


(a) $K = 2$ (b) $K = 128$

Figure 2: Node classification performance of gfSGC on Cora with varying $\lambda$ and $K$.
