# Supplementary material for: Simple yet Effective Gradient-Free Graph Convolutional Networks
Source: arXiv:2302.00371 source file (2023-02-01)
Supplement: Supplementary file 2 [file appendix.tex]

\appendix
\section{Vanishing Gradient of Large $K$}
Recall the feed-forward formula Eqn.~\eqref{general-sgc} of linearized GCN,
\begin{equation}
    \widehat{\mathbf{Y}}=\text{softmax}(\mathcal{F}_{G}\mathbf{W}),
\end{equation}
which is trained by minimizing cross-entropy loss,
\begin{equation}
    \min \mathcal{L}_{CE}{(\mathbf{Y}, \widehat{\mathbf{Y}})}.
\end{equation}
By the chain rule, we have
\begin{equation}
    \frac{\partial \mathcal{L}_{CE}}{\partial \mathbf{W}} = \mathcal{F}_{G}^\top \frac{\partial \mathcal{L}_{CE}}{\partial \mathbf{H}}, 
\end{equation}
where $\mathbf{H}\overset{\Delta}{=}\mathcal{F}_{G}\mathbf{W}$. The gradient of parameter $\mathbf{W}$ is greatly affected by the scale of $\mathcal{F}_{G}$. Parameter $\mathbf{W}$ suffers from the vanishing gradient problem if $\mathcal{F}_{G}$ is too small. However, this is true when $K$ is large. 

Since the existence of bias parameters in neural networks, neural networks are invariant to data point translation, so we discuss the scale of zero-centered $\mathcal{F}_{G}$:
\begin{equation}
    F_G - \frac1N\mathbf{1}_N\mathbf{1}_N^\top\mathcal{F}_{G},
\end{equation}
where $\mathbf{1}_N\in\mathbbm{R}^{N}$ is an all-one vector, and $\frac1N\mathbf{1}_N^\top\mathcal{F}_{G}$ is the center of data points. 
When $K$ approximates $+\infty$, zero-centered $\mathcal{F}_{G}$ approximates a zero vector for SGC with row-normalized adjacency matrix $A_{rw}=\mathbf{D}^{-1}\mathbf{A}$, if the graph is connected and not a bipartite.
\begin{equation}\label{eq:sgc_dgc_lim}
\lim_{K\to\infty} \left(\mathcal{F}_{G} - \frac1N\mathbf{1}_N\mathbf{1}_N^\top\mathcal{F}_{G}\right) = \mathbf{0}
\end{equation}

For DGC, it approximates 
\begin{equation}
    \lim_{K\to\infty} \left(\mathcal{F}_{G} - \frac1N\mathbf{1}_N\mathbf{1}_N^\top\mathcal{F}_{G}\right) =
\end{equation}

For SSGC, it approximates zero-centered $\tau \mathbf{X}$, which is small if $\tau$ is small.
\begin{equation}\label{eq:ssgc_lim}
\lim_{K\to\infty} \left(\mathcal{F}_{G} - \frac1N\mathbf{1}_N\mathbf{1}_N^\top\mathcal{F}_{G}\right) =
    \tau \left(\mathbf{X} - \frac1N\mathbf{1}_N\mathbf{1}_N^\top\mathbf{X}\right)
\end{equation}
\begin{proof}
If the graph is connected and not a bipartite, the greatest eigenvalue of $A_{\text{rw}}$ is 1, and the corresponding eigenvector is $\mathbf{1}_N$. All eigenvalues of the $A_{\text{rw}}$ other than 1 falls into range $(-1, 1)$. For SGC, when $K$ approximates $+\infty$, only component of eigenvector $\mathbf{1}_N$ in $\mathbf{X}$ is reserved, so
\begin{equation}\label{eq:sgc_lim}
    \lim_{K\to\infty} \mathcal{F}_{G} = \lim_{K\to\infty} \mathbf{A}_{rw}^K\mathbf{X} = \theta \mathbf{1}_{N}\mathbf{1}_C^\top.
\end{equation}
For DGC, $\mathcal{F}_{G} = \mathbf{A}_{dgc}^K \mathbf{X}$, where
\begin{equation}
    \mathbf{A}_{dgc}=\left(1-\tfrac{T}{K}\right)I+\tfrac{T}{K}\hat{\mathbf{A}}_{rw}.
\end{equation}
Similarly, the greatest eigenvalue of $\mathbf{A}_{dgc}$ is 1, and the corresponding eigenvector is $\mathbf{1}_N$. All other eigenvalues of $\mathbf{A}_{dgc}$ other than 1 falls into range $(-1, 1)$, so
\begin{equation}\label{eq:dgc_lim}
    \lim_{K\to\infty} \mathcal{F}_{G} = \lim_{K\to\infty} \mathbf{A}_{dgc}^K \mathbf{X} = \theta \mathbf{1}_{N}\mathbf{1}_C^\top.
\end{equation}
Given Eqn. \eqref{eq:sgc_lim} and \eqref{eq:dgc_lim}, it is easy to verify that Eqn. \eqref{eq:sgc_dgc_lim} holds. Although zero-centered $\mathcal{F}_G$ of both SGC and DGC converge to zero vector, DGC converges much slower than SGC.

For SSGC, we have
\begin{equation}
    \mathcal{F}_G = \tau \mathbf{X} + (1-\tau) \frac1K \sum_{k=1}^K \mathbf{A}^k_{rm} \mathbf{X}.
\end{equation}
By Eqn. \eqref{eq:sgc_lim},
\begin{equation}
    \lim_{K\to\infty} \mathcal{F}_{G} = \tau \mathbf{X} + (1-\tau) \theta \mathbf{1}_{N}\mathbf{1}_C^\top.
\end{equation}
So, Eqn \eqref{eq:ssgc_lim} holds. The right side of \eqref{eq:ssgc_lim} is just the zero-centered $\tau \mathbf{X}$.
\end{proof}
Above analysis applies to row-normalized adjacency matrix $\mathbf{A}_{rw}$, while the most commonly adopted one is symmetrically normalized $\hat{\mathbf{A}}$. For $\hat{\mathbf{A}}$ symmetrically normalized, the left side of Eqn. \eqref{eq:sgc_dgc_lim} converges to a small vector instead of zero, so vanishing gradients still exist.

\section{Scale invariant of problem \eqref{eqn-OLS}}
% \begin{equation}
% \mathcal{L}_{MSE} = (\mathbf{Y}-\Phi(\mathcal{F}_{G})\mathbf{W})^\top(\mathbf{Y}-\Phi(\mathcal{F}_{G})\mathbf{W})+\xi\Tr(\mathbf{W}^\top\mathbf{W})
% \end{equation}

The optimization problem \eqref{eqn-OLS} has following closed-form solution,
\begin{equation}
\mathbf{W}^* = \left(\Phi(\mathcal{F}_{G})^\top \Phi(\mathcal{F}_{G}) + \xi I\right)^{-1}\Phi(\mathcal{F}_{G})^\top \mathbf{Y}.
\end{equation}
The optimal solution $\mathbf{W}^*$ results in an estimation $\widehat{\mathbf{Y}}^*$,
\begin{equation}
\begin{split}
    \widehat{\mathbf{Y}}^*
        & = \Phi(\mathcal{F}_{G})\mathbf{W}^* \\
        & = \Phi(\mathcal{F}_{G})\left(\Phi(\mathcal{F}_{G})^\top \Phi(\mathcal{F}_{G}) + \xi I\right)^{-1}\Phi(\mathcal{F}_{G})^\top \mathbf{Y}.
\end{split}
\end{equation}
We consider $\widehat{\mathbf{Y}}^*$ as a function of $\Phi(\mathcal{F}_{G})$ and $\xi$,
\begin{equation}
    \widehat{\mathbf{Y}}^* = \widehat{\mathbf{Y}}^*(\Phi(\mathcal{F}_{G}), \xi).
\end{equation}
If we scale $\Phi(\mathcal{F}_{G})$ by a constant $\beta$, and scale $\xi$ by $\beta^2$, the estimation $\widehat{\mathbf{Y}}^*$ is invariant, i.e.,
\begin{equation}
    \widehat{\mathbf{Y}}^* (\Phi(\mathcal{F}_{G}), \xi) = \widehat{\mathbf{Y}}^* (\beta \Phi(\mathcal{F}_{G}), \beta^2 \xi).
\end{equation}
In other words, the estimator resulting from the optimization problem \eqref{eqn-OLS} is invariant to the scale of $\Phi(\mathcal{F}_{G})$, as long as hyper-parameter $\xi$ is properly scaled correspondingly. This also tells us that when $K$ is large, and the scale of $\Phi(\mathcal{F}_{G})$ is small, we should use small $\xi$.
